# Supplementary material for: Picosecond creation of switchable optomagnets with giant photoinduced Kerr rotations in polar antiferromagnetic (Fe$_{1-x}$Zn$_{x}$)$_{2}$Mo$_{3}$O$_{8}$
Source: arXiv:2109.03498 source file (2021-09-08)
Supplement: Supplementary file 1 [file SupplMat_FMO.pdf]

# Supplemental material for "Picosecond creation of switchable optomagnets from a polar antiferromagnet with giant photoinduced Kerr rotations"

Y. M. Sheu,<sup>1,2</sup> Y. M. Chang,<sup>1</sup> C. P. Chang,<sup>1</sup> Y. H. Li,<sup>1</sup> K.  
R. Babu,<sup>3,4</sup> G.Y. Guo,<sup>3,4</sup> T. Kurumaji,<sup>5</sup> and Y. Tokura<sup>6,7</sup>

<sup>1</sup>*Department of Electrophysics, National Chiao Tung University, Hsinchu, 30010, Taiwan*

<sup>2</sup>*Center for Emergent Functional Matter Science,*

*National Chiao Tung University, Hsinchu 30010, Taiwan*

<sup>3</sup>*Department of Physics and Center for Theoretical Physics,*

*National Taiwan University, Taipei, 10617, Taiwan*

<sup>4</sup>*Physics Division, National Center for Theoretical Sciences, Hsinchu 30013, Taiwan*

<sup>5</sup>*Department of Physics, Massachusetts Institute*

*of Technology, Cambridge, MA 02139-4307, USA*

<sup>6</sup>*RIKEN Center for Emergent Matter Science (CEMS), Wako, Saitama 351-0198, Japan*

<sup>7</sup>*Department of Applied Physics, University of Tokyo, Tokyo 113-8656, Japan*

## I. AB INITIO CALCULATIONS

To better understand the experimental results related to various absorption features and magnetic interactions, we perform *ab initio* electronic structure calculations for the pure  $\text{Fe}_2\text{Mo}_3\text{O}_8$  based on density functional theory with the generalized gradient approximation (GGA) [S1]. Strong Fe *d*-orbital Coulomb interaction is further taken into account by using the GGA plus on-site Coulomb interaction (GGA+*U*) scheme [S2]. A reasonable effective *U* of 5 eV is used for Fe *d*-orbitals [S3]. The accurate projector-augmented wave band structure method, implemented in the VASP code [S4, S5], together with a large

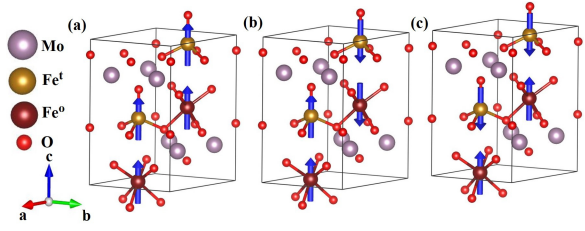

FIG. S1: Crystalline structure of  $\text{Fe}_2\text{Mo}_3\text{O}_8$  with (a) ferromagnetic (FM), (b) antiferromagnetic (AFM) and (c) ferrimagnetic (FRM) configurations. The vertical blue arrows indicate the Fe magnetic moment directions.

plane-wave cut-off energy of 480 eV, is used.

Pure  $\text{Fe}_2\text{Mo}_3\text{O}_8$  crystalizes in the hexagonal  $P6_3mc$  structure with 2 formula units (f.u.) per unit cell (see Fig. S1) [S6]. In the present calculations, a  $\Gamma$ -centered k-point mesh of  $8 \times 8 \times 4$  is used for the Brillouin zone integration, and the self-consistency criterion is the total energy convergence within  $10^{-6}$  eV. We consider ferromagnetic (FM) as well as antiferromagnetic (AFM) and ferrimagnetic (FRM) orders [S7] (see Fig. S1). We start structural optimization calculations with the use of experimental lattice constants  $a = 5.7732$  Å and  $c = 10.054$  Å [S6]. We find that the AFM state has the lowest total energy (see Table S1) with the theoretical lattice constants  $a = 5.775$  Å and  $c = 10.048$  Å, being in good agreement with the experimental values [S6]. Therefore, from now on, we focus on the properties of the AFM state (see Fig. S1(b)). The calculated spin magnetic moments are  $3.79 \mu_B$  on the tetrahedral Fe site and  $3.92 \mu_B$  on the octahedral Fe site (Table S1). These magnetic moments are close to  $4.0 \mu_B$  expected for the  $\text{Fe}^{2+} d^6$  ( $t_{2g}^3 \uparrow e_g^2 \uparrow t_{2g}^1 \downarrow$ ) and  $\text{Fe}^{2+} d^6$  ( $t_{2g}^3 \uparrow e_g^2 \uparrow e_g^1 \downarrow$ ) ionic configurations on the octahedral and tetrahedral sites, respectively.

To understand the AFM ground state and also determine the near neighboring exchange coupling parameters among the Fe atoms, we further perform the self-consistent total energy calculations for three more AFM configurations, as shown in Fig. S2. The calculated Fe spin magnetic moments and total energies are also listed in Table S1.

TABLE S1: Calculated total energies ( $\Delta E$ ), octahedral and tetrahedral Fe spin magnetic moments ( $m_s^o$ ,  $m_s^t$ ) of various considered magnetic configurations (see Figs. S1 and S2) of pure  $\text{Fe}_2\text{Mo}_3\text{O}_8$ . The total energies are relative to the total energy of the FM configuration.

|      | $\Delta E$ (meV/f.u.) | $m_s^o$ ( $\mu_B$ ) | $m_s^t$ ( $\mu_B$ ) |
|------|-----------------------|---------------------|---------------------|
| FM   | 0.0                   | 3.94                | 3.80                |
| AFM  | -52.9                 | 3.92                | 3.79                |
| FRM  | -28.3                 | 3.91                | 3.77                |
| AFM2 | -17.2                 | 3.93                | 3.80                |
| AFM3 | -8.8                  | 3.92                | 3.79                |
| AFM4 | -1.2                  | 3.93                | 3.79                |

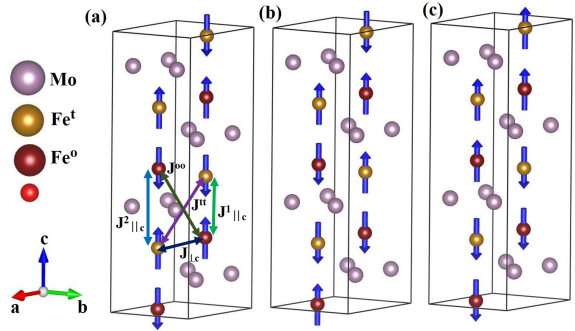

FIG. S2:  $1 \times 1 \times 2$  supercell structure of  $\text{Fe}_2\text{Mo}_3\text{O}_8$  with (a) antiferromagnetic 2 (AFM2), (b) 3 (AFM3) and (c) 4 (AFM4) configurations. The vertical blue arrows indicate the Fe magnetic moment directions. The first 5 near neighbor exchange coupling parameters ( $J_{\perp c}$ ,  $J_{\parallel c}^1$ ,  $J_{\parallel c}^2$ ,  $J_{tt}$ ,  $J_{oo}$ ) are indicated in (a) and their values are listed in Table S2.

We then evaluate the exchange coupling parameters by mapping the calculated total energies of different magnetic configurations onto the classical Heisenberg Hamiltonian,  $E = E_0 - \sum_{i,j} J_{ij} \hat{\mathbf{e}}_i \cdot \hat{\mathbf{e}}_j$ , where  $E_0$  donates the nonmagnetic ground state energy;  $J_{ij}$  the

TABLE S2: Calculated various exchange coupling parameters ( $J_{\perp c}$ ,  $J_{\parallel c}^1$ ,  $J_{\parallel c}^2$ ,  $J_{\text{tt}}$ ,  $J_{\text{oo}}$ ) (see Fig. S2 (a)) of pure  $\text{Fe}_2\text{Mo}_3\text{O}_8$ .  $J_{\parallel c} = (J_{\parallel c}^1 + J_{\parallel c}^2)/2$ . The corresponding Fe-Fe distances ( $d_{\text{Fe-Fe}}$ ) are also listed.

|                     | $d_{\text{Fe-Fe}}$ (Å) | $J_{ij}$ (meV) |
|---------------------|------------------------|----------------|
| $J_{\perp c}$       | 3.3893                 | -9.2           |
| $J_{\parallel c}^1$ | 4.4126                 | 1.3            |
| $J_{\parallel c}^2$ | 5.6415                 | 2.6            |
| $J_{\parallel c}$   | 5.0271                 | 2.0            |
| $J_{\text{tt}}$     | 6.0317                 | -4.3           |
| $J_{\text{oo}}$     | 6.0317                 | -4.1           |

exchange coupling parameter between sites  $i$  and  $j$ ;  $\hat{\mathbf{e}}_i$ , the unit vector representing the direction of the magnetic moment on site  $i$ . The exchange coupling parameters derived this way are listed in Table S2, together with the corresponding Fe-Fe distances. As can be expected from the AFM ground state, Table S2 shows that intralayer magnetic coupling between the nearest neighbors ( $J_{\perp c}$ ) is antiferromagnetic (negative) and is strongest. This is also consistent with the fact that when the magnetic moment of the octahedral Fe site is flipped upwards by the external magnetic field, the magnetic moment on the tetrahedral Fe site is also flipped (but downwards) (see the second layer in Figs. S1(b) and S1(c)), thus resulting in the FRM configuration (Fig. S1(c)). The vertical interlayer magnetic couplings between the octahedral and tetrahedral Fe atoms ( $J_{\parallel c}^1$  and  $J_{\parallel c}^2$ ), on the other hand, are ferromagnetic (positive). The nearest-neighbor exchange couplings between the octahedral Fe atoms ( $J_{\text{oo}}$ ) and between the tetrahedral ( $J_{\text{tt}}$ ) Fe atoms are both antiferromagnetic (negative) and have almost the same values (Table S2). These two findings are also consistent with the AFM ground state (Fig. S1(b)).

The calculated AFM band structure is displayed in Fig. S3, and the corresponding total and orbital-decomposed densities of states (DOSs) which are calculated using a denser k-point mesh of  $16 \times 16 \times 8$ , are plotted in Fig. S4. It is clear that the electronic band structure consists of three band regions, namely, the 8 conduction band manifold made of mainly Mo *d*-orbital and tetrahedral Fe *d*-orbital hybridized bands in the vicinity of the Fermi level, the valence band manifold lying about 1.2 eV below the Fermi level, and the higher conduction band region lying about 1.5 eV above the Fermi level. Figure S3 shows that the system is a semimetal with the lowest conduction band and highest valence band touching along the  $\Gamma$ –A symmetry line in the Brillouin zone. However, when the spin-orbit coupling is included, the highest valence band splits off and the system becomes an insulator with a band gap of about 1.41 eV. The 5 Fe *d*-orbitals would split into doubly degenerate  $e_g$  and triply degenerate  $t_{2g}$  states in the ideal octahedral and tetrahedral coordination. Nonetheless, in  $\text{Fe}_2\text{Mo}_3\text{O}_8$ , both the octahedral and tetrahedral Fe sites have the  $C_{3v}$  site symmetry and consequently, the 5 Fe *d*-orbitals would further regroup into two doubly degenerate  $E_g$  states  $[(d_{x^2-y^2}, d_{xy}), (d_{xz}, d_{yz})]$  and one nondegenerate  $A_g$  state ( $d_{z^2}$ ) (Fig. S4). By examining the calculated orbital characters of the conduction bands at the  $\Gamma$ -point, we are able to locate these Fe *d*-orbital dominated states, and hence we are able to estimate the one-electron Fe *d*-*d* excitation energies. We find that for the octahedral Fe, the excitation energies of  $t_{2g} \rightarrow e_g$  transitions below the absorption edge are 1.01 and 1.19 eV and that for the tetrahedral Fe, the excitation energies are 0.54 and 1.14 eV, as marked Fig. S5 below the optical absorption edge.

We calculate the absorption spectrum due to the interband transitions from the relativistic band structure by using the Fermi golden rule (see, e.g., Ref. [S8]), and the result is shown in Fig. S5. It is clear that the calculated absorption spectrum agree rather well with the measured *p*-*d* transition spectrum. Figure S5 also shows that the estimated Fe *d*-*d* excitation energies are also in reasonably good agreement with the experimental

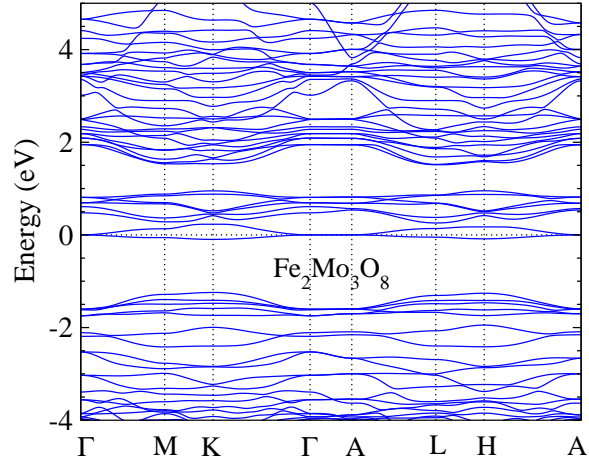

FIG. S3: Calculated band structure of  $\text{Fe}_2\text{Mo}_3\text{O}_8$ . The Fermi level is at 0 eV.

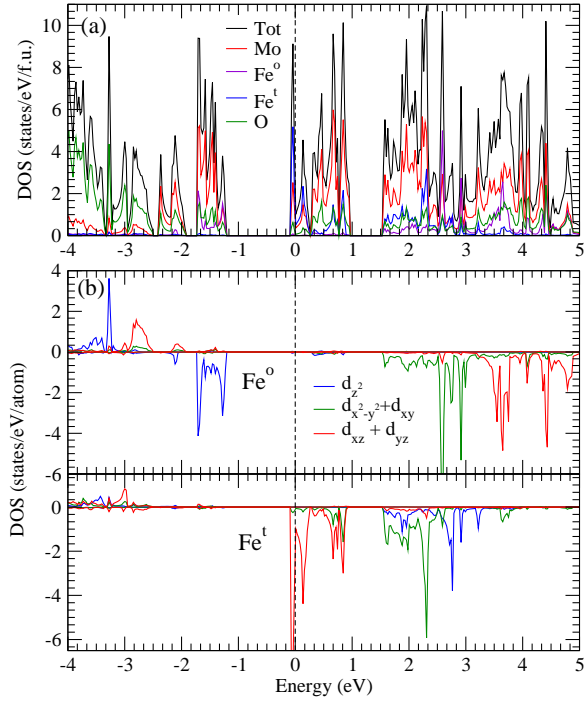

FIG. S4: Calculated total, site- and orbital-decomposed density of states (DOS) of  $\text{Fe}_2\text{Mo}_3\text{O}_8$ .

values.

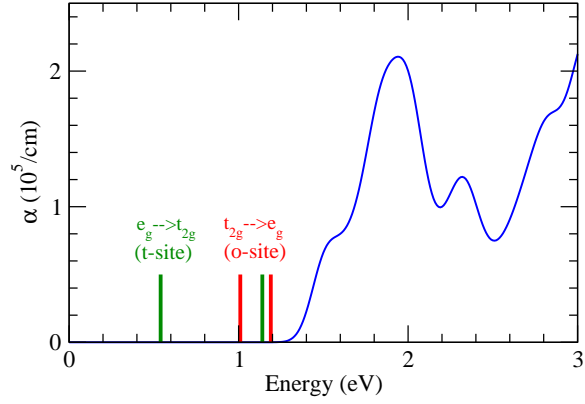

FIG. S5: Calculated optical absorption spectrum ( $\alpha$ ) of  $\text{Fe}_2\text{Mo}_3\text{O}_8$  due to direct interband transitions, together with the pre-absorption edge Fe d-d transition energies marked by the vertical lines. The absorption spectrum is obtained from the relativistic band structure with the inclusion of spin-orbit coupling, giving rise to a semiconducting band gap of 1.41 eV.

## II. DISAPPEARANCE OF THE GIANT KERR ROTATIONS FOR $x=0.125$ IN THE PARAMAGNETIC PHASE

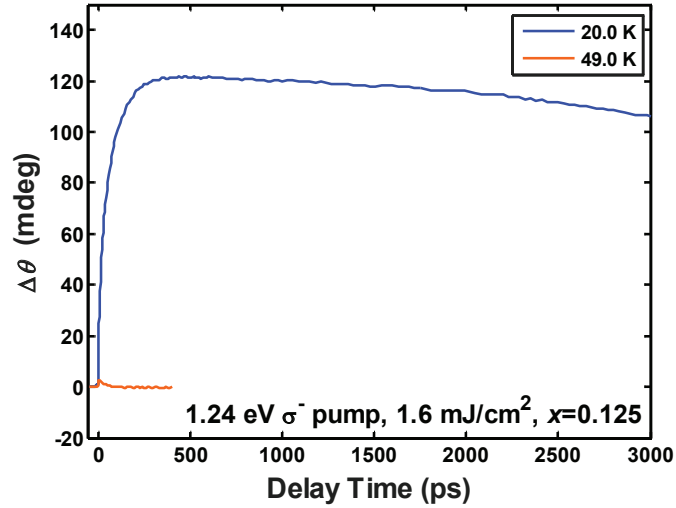

FIG. S6: For  $x=0.125$ , the giant photoinduced magnetization disappears in the paramagnetic phase above 48 K.

### III. ENHANCEMENT OF TRMOKE FROM THE T-SITE D-D TRANSITION

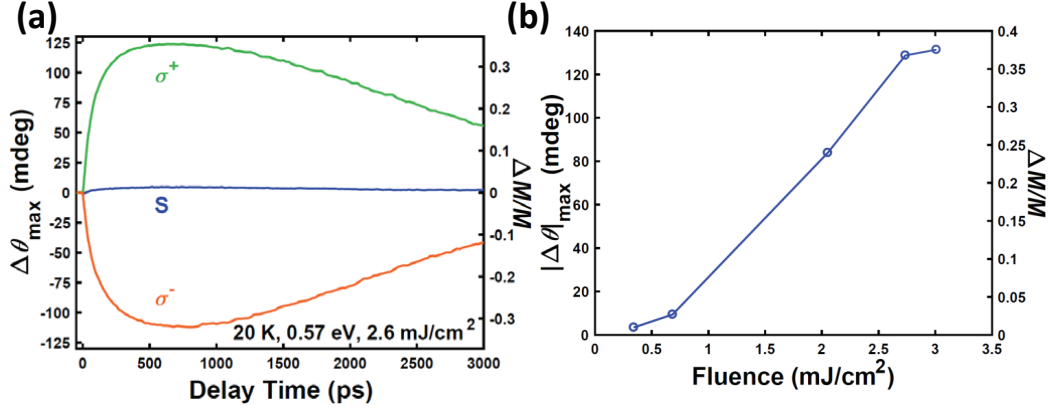

FIG. S7: (a) Giant enhancement of time-resolved magneto-optical Kerr rotation (TRMOKE) is also observed from the T-site  $d-d$  transition (0.57eV,  $T_{d-d}$ ) in the sample with 12.5% doping concentration ( $x=0.125$ ). The polarity of TRMOKE here is also controllable by light helicity. (b) The maximum Kerr rotation versus pump fluence from  $T_{d-d}$  at 20 K. The fluence we can achieve in the  $T_{d-d}$  measurement is significantly reduced due to the instrumentation limit at longer laser wavelength. The right axis of both figure displays the photoinduced magnetization, which is calibrated as described in Appendix A of the main text.

Time-resolved magneto-optical Kerr effect (TRMOKE) displays the same behavior between excitation from the T-site  $d-d$  transition (0.57 eV,  $T_{d-d}$ , Fig. S7(a)) and excitation from the O-site  $d-d$  transition (1.24 eV,  $O_{d-d}$ , shown in Fig. 4 of the main text). The only difference observed is the opposite polarity of Kerr rotation when the same light helicity is employed to excite these two transitions, consistent with our observation from  $\text{Fe}_2\text{Mo}_3\text{O}_8$  without Zn doping. This is again analogous to the field flip for each site, with the exception that only the selective sublattice flips spin directly via using light helicity. The maximum Kerr rotation versus pump fluence from  $T_{d-d}$ , Fig. S7(b), displays the same behavior as that from  $O_{d-d}$  as well, indicating their same

mechanism that leads to the giant enhancement of TRMOKE, as elaborated in the main text.

- 
- [S1] J. P. Perdew, K. Burke, and M. Ernzerhof, Phys. Rev. Lett. **77**, 3865 (1996).
  - [S2] S. L. Dudarev, G. A. Botton, S. Y. Savrasov, C. J. Humphreys, and A. P. Sutton, Phys. Rev. B **57**, 1505 (1998).
  - [S3] H.-T. Jeng, G. Y. Guo, and D. J. Huang, Phys. Rev. Lett. **93**, 156403 (2004).
  - [S4] G. Kresse and J. Hafner, Phys. Rev. B **47**, 558 (1993).
  - [S5] G. Kresse and J. Furthmüller, Comput. Mater. Sci. **6**, 15 (1996).
  - [S6] Y. Le Page and P. Strobel, Acta Cryst. B **38**, 1265 (1982).
  - [S7] Y. Wang, G. L. Pascut, B. Gao, T. A. Tyson, K. Haule, V. Kiryukhin, and S.-W. Cheong, Sci. Rep. **5**, 12268 (2015).
  - [S8] G. Y. Guo, K. C. Chu, D.-S. Wang, and C.-G. Duan, Phys. Rev. B **69**, 205416 (2004).
